# Supplementary material for: Fast and Lightweight Backdoor Detection via Head Random Probing
Source: arXiv:2605.18908 source file (2026-05-17)
Supplement: Supplementary file 1 [file 7.appendix.tex]

\begin{figure*}
    \centering
\begin{minipage}[c]{1\textwidth}
    \centering
    \includegraphics[width=0.7\textwidth]{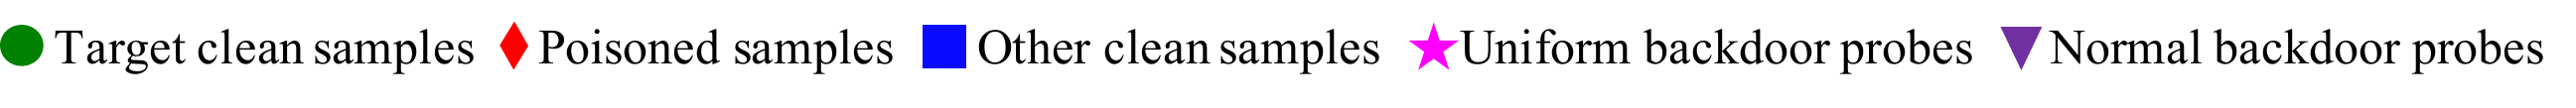}
  \end{minipage}
  \vspace{-7mm}

\begin{minipage}[c]{0.02\textwidth}
\vspace{14mm}
\rotatebox{90}{
\begin{tcolorbox}[
        colback=white, % 背景颜色
        colframe=white, % 边框颜色
    ]{\footnotesize Badnet}
\end{tcolorbox}}
\end{minipage}
\begin{minipage}[c]{0.972\textwidth}
    \centering
    \subfloat[GNet]{\includegraphics[width=0.14\textwidth]{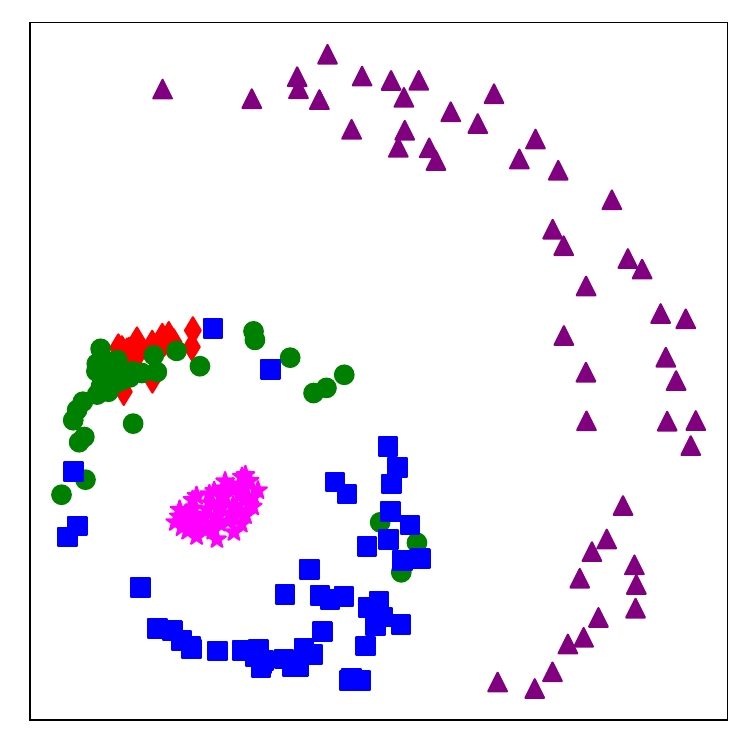}}
    \subfloat[R18]{\includegraphics[width=0.14\textwidth]{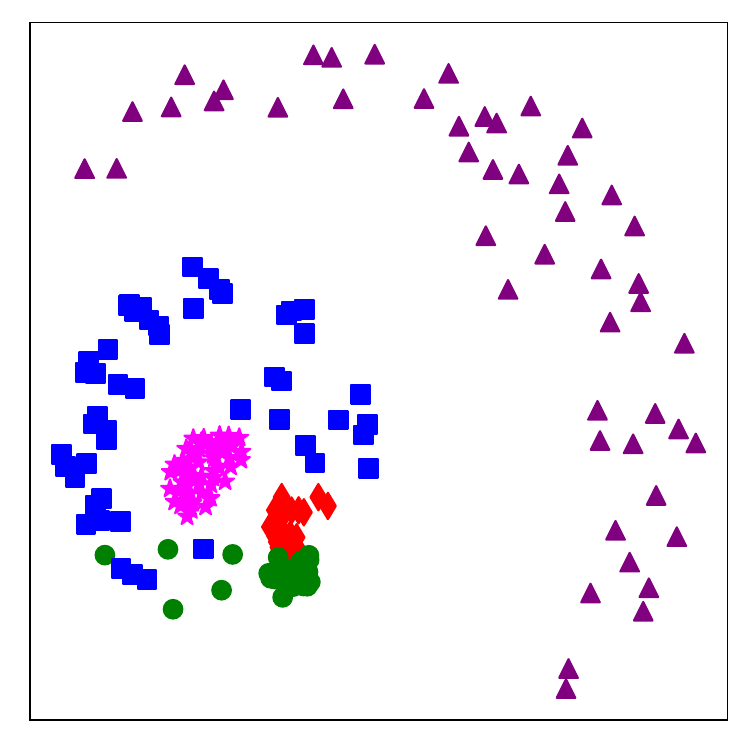}}
    \subfloat[V16]{\includegraphics[width=0.14\textwidth]{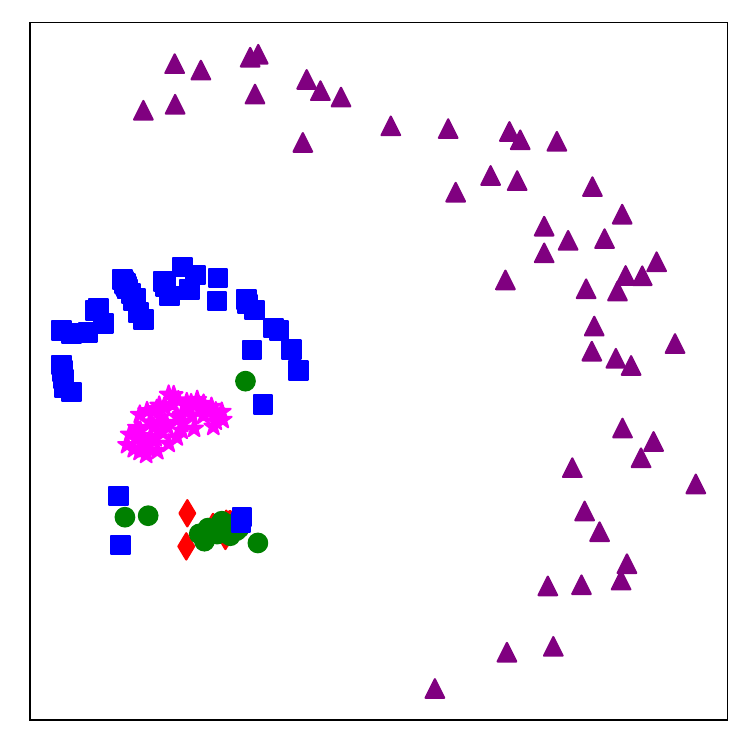}}
    \subfloat[SNet]{\includegraphics[width=0.14\textwidth]{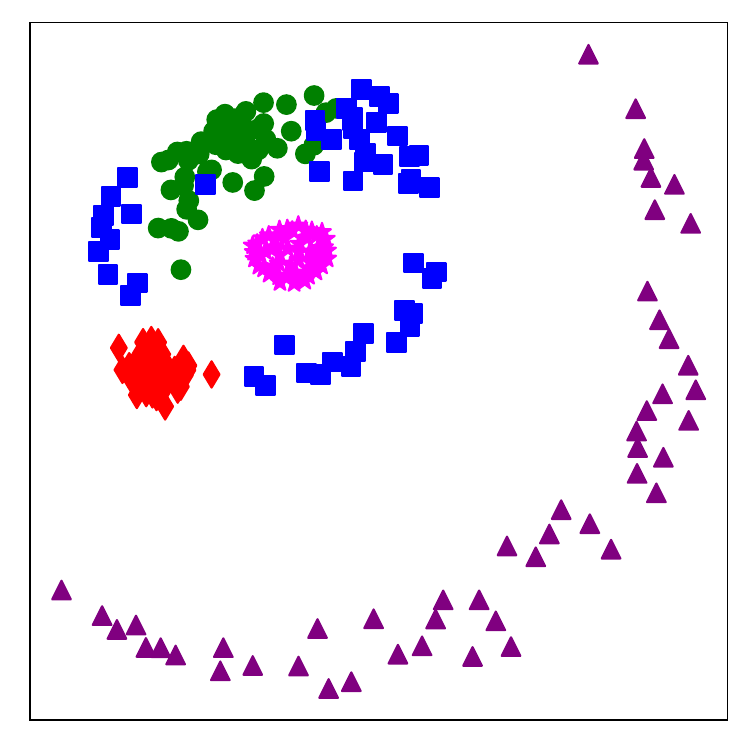}}
    \subfloat[PR18]{\includegraphics[width=0.14\textwidth]{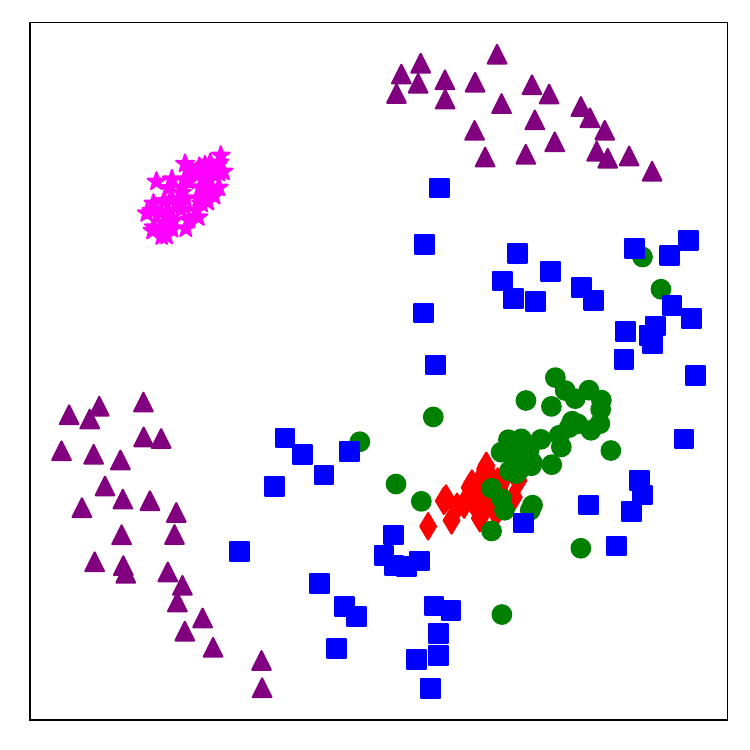}}
    \subfloat[CNN6]{\includegraphics[width=0.14\textwidth]{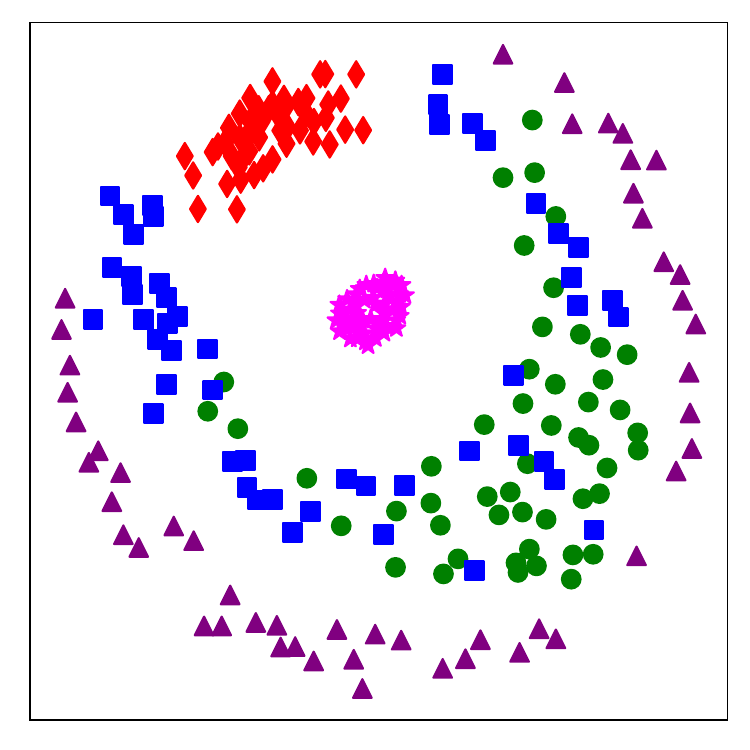}}
    \subfloat[ENet]{\includegraphics[width=0.14\textwidth]{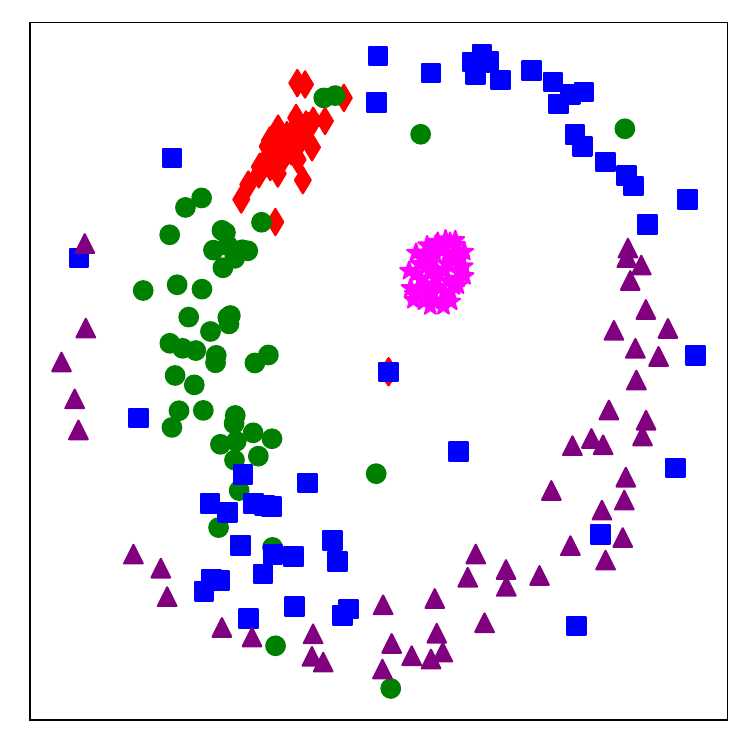}}
  \end{minipage}
  % \vspace{-2mm}

% \begin{minipage}[c]{0.02\textwidth}
% \vspace{14mm}
% \rotatebox{90}{
% \begin{tcolorbox}[
%         colback=white, % 背景颜色
%         colframe=white, % 边框颜色
%     ]{\footnotesize Blended}
% \end{tcolorbox}}
% \end{minipage}
%  \begin{minipage}[c]{0.972\textwidth}
%     \centering
%     \subfloat[GNet]{\includegraphics[width=0.14\textwidth]{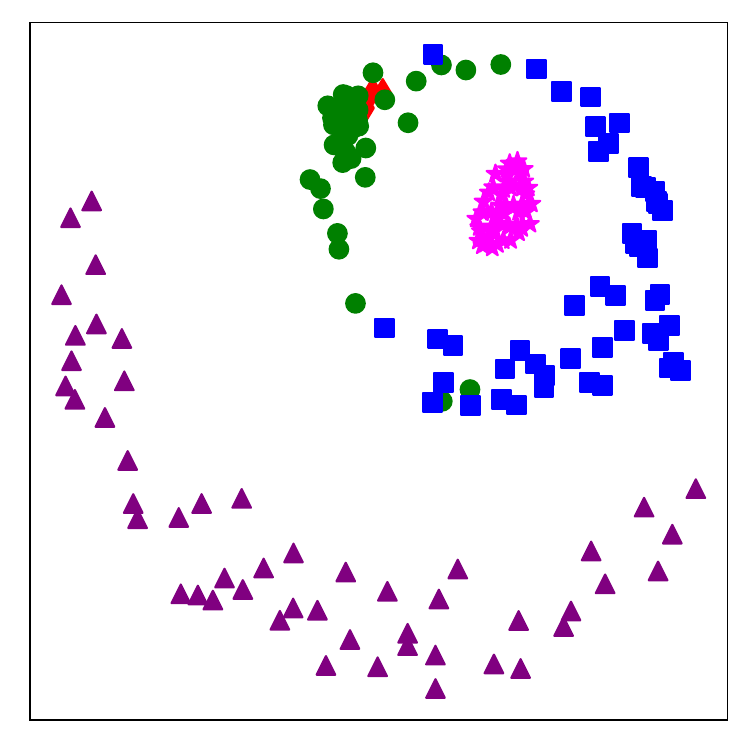}}
%     % \hspace{0.005\textwidth}
%     \subfloat[R18]{\includegraphics[width=0.14\textwidth]{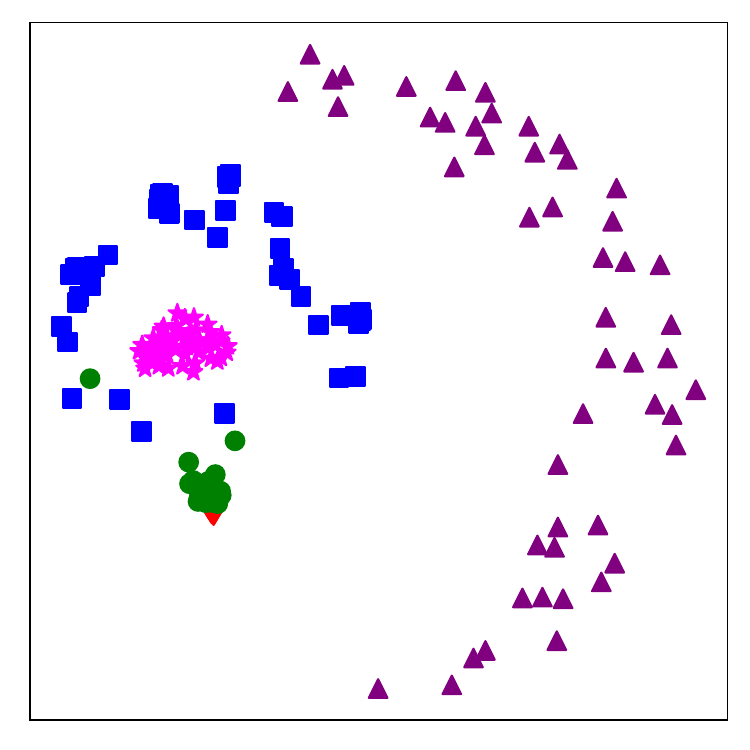}}
%     % \hspace{0.005\textwidth}
%     \subfloat[V16]{\includegraphics[width=0.14\textwidth]{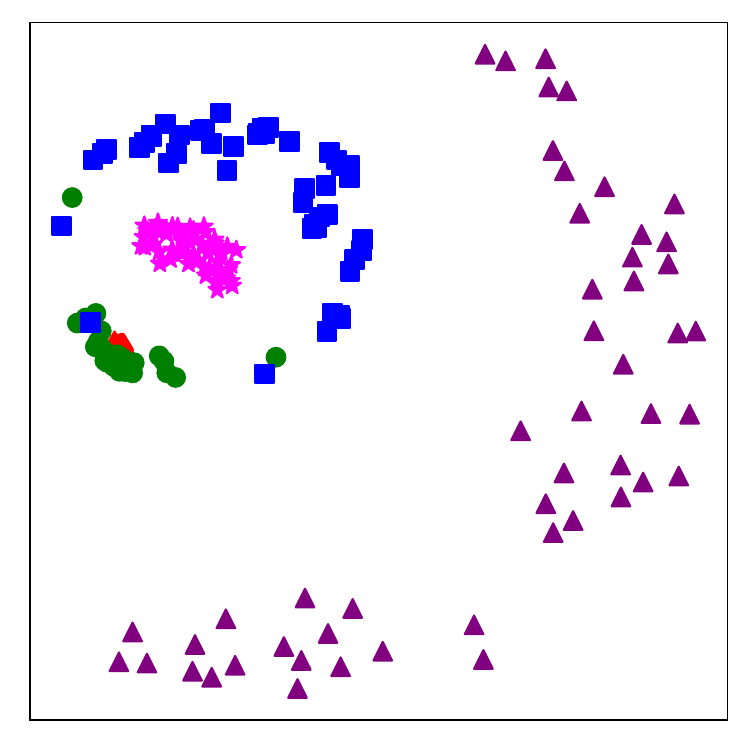}}
%     \subfloat[SNet]{\includegraphics[width=0.14\textwidth]{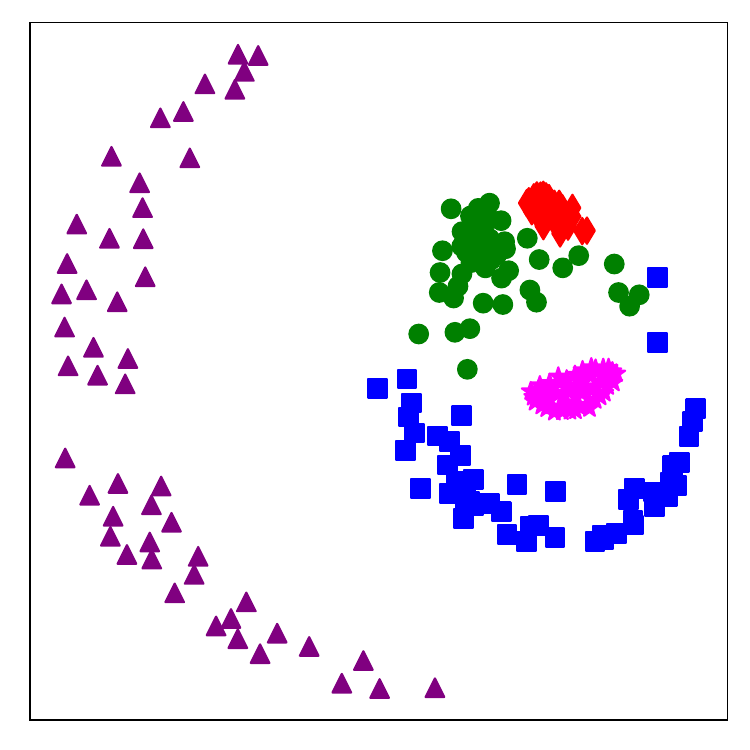}}
%     \subfloat[PR18]{\includegraphics[width=0.14\textwidth]{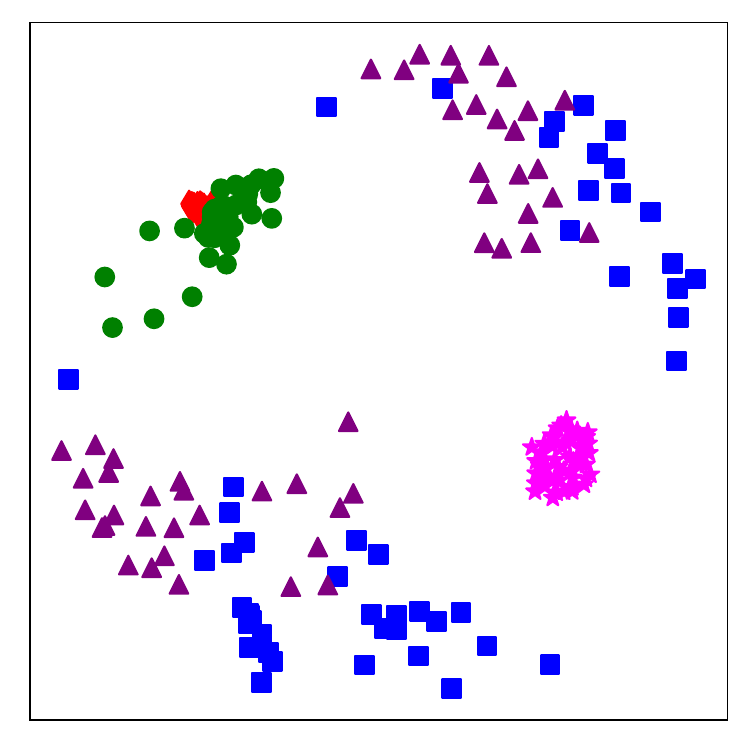}}
%     \subfloat[CNN6]{\includegraphics[width=0.14\textwidth]{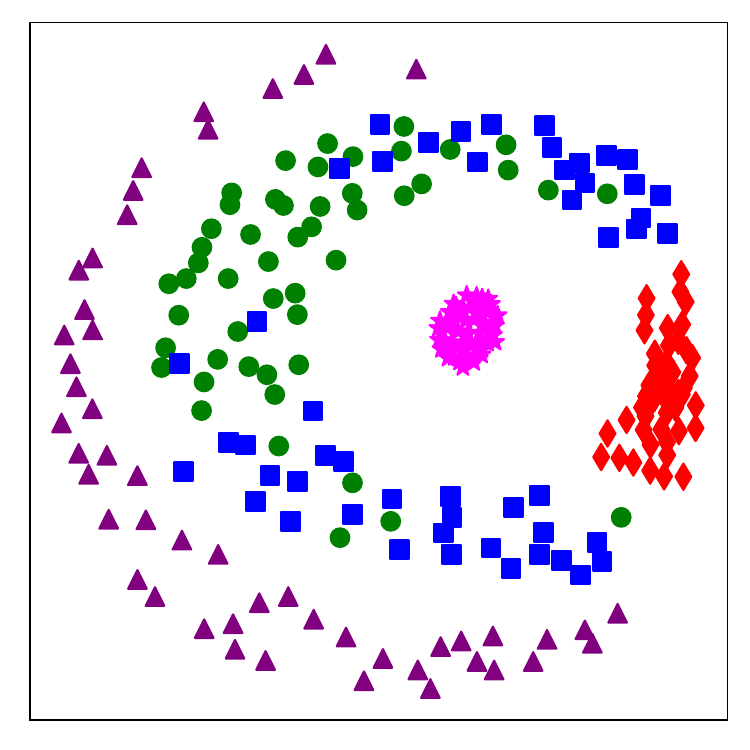}}
%     \subfloat[ENet]{\includegraphics[width=0.14\textwidth]{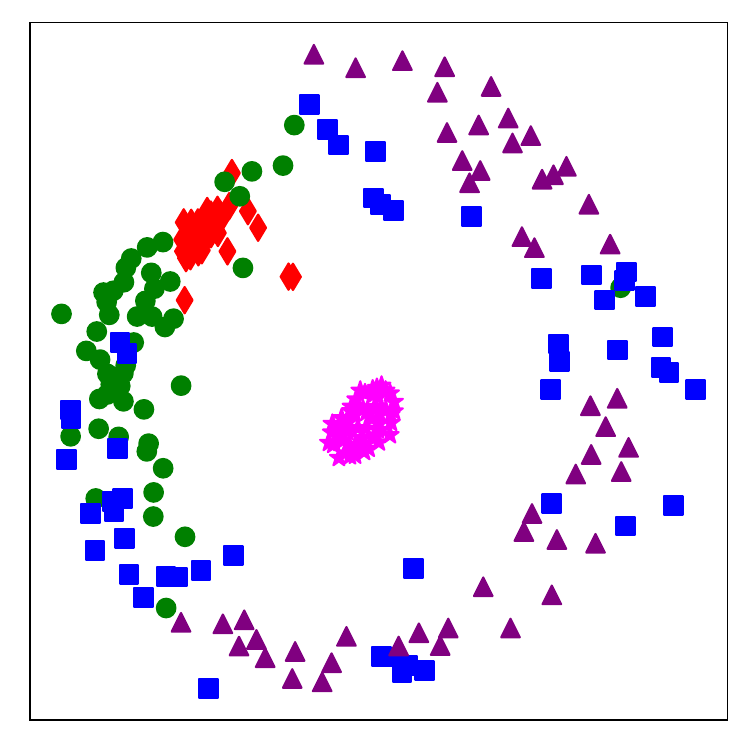}}
%   \end{minipage}
  % \vspace{-2mm}

\begin{minipage}[c]{0.02\textwidth}
\vspace{14mm}
\rotatebox{90}{
\begin{tcolorbox}[
        colback=white, % 背景颜色
        colframe=white, % 边框颜色
    ]{\footnotesize ISSBA}
\end{tcolorbox}}
\end{minipage}
 \begin{minipage}[c]{0.972\textwidth}
    \centering
    \subfloat[GNet]{\includegraphics[width=0.14\textwidth]{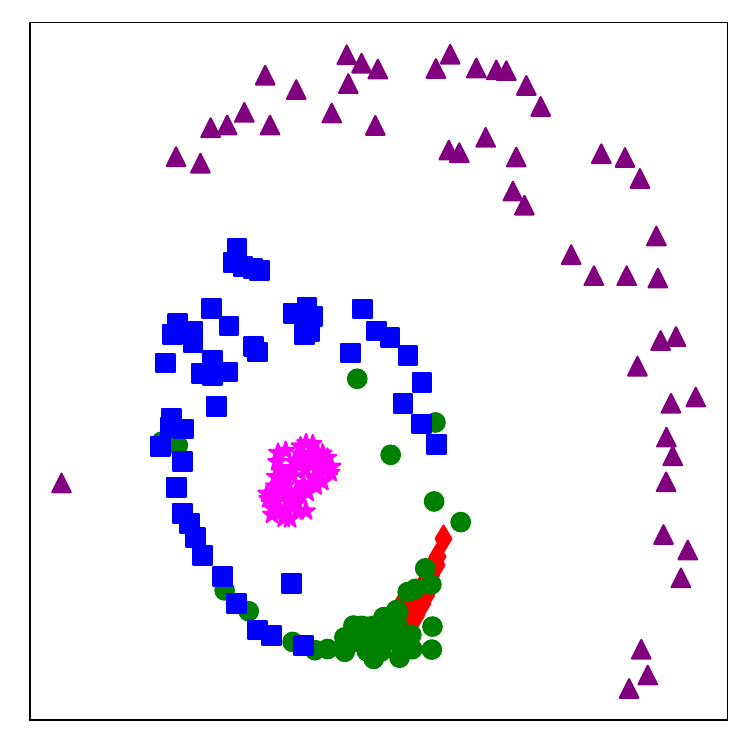}}
    % \hspace{0.005\textwidth}
    \subfloat[R18]{\includegraphics[width=0.14\textwidth]{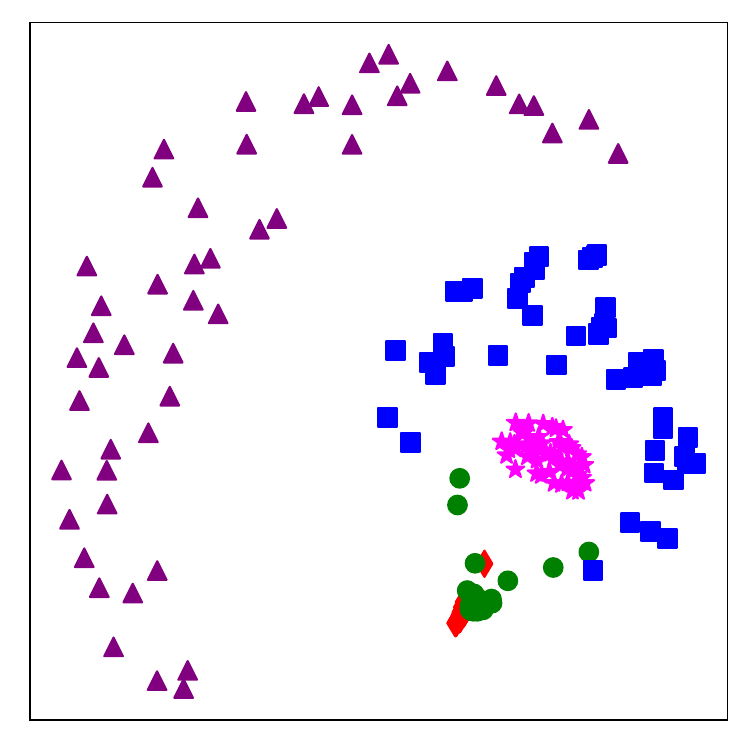}}
    % \hspace{0.005\textwidth}
    \subfloat[V16]{\includegraphics[width=0.14\textwidth]{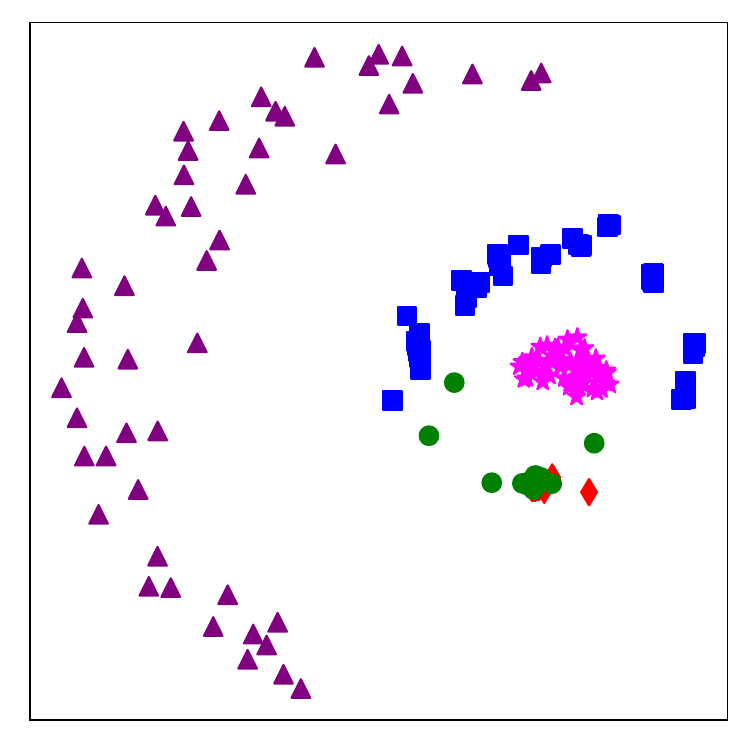}}
    \subfloat[SNet]{\includegraphics[width=0.14\textwidth]{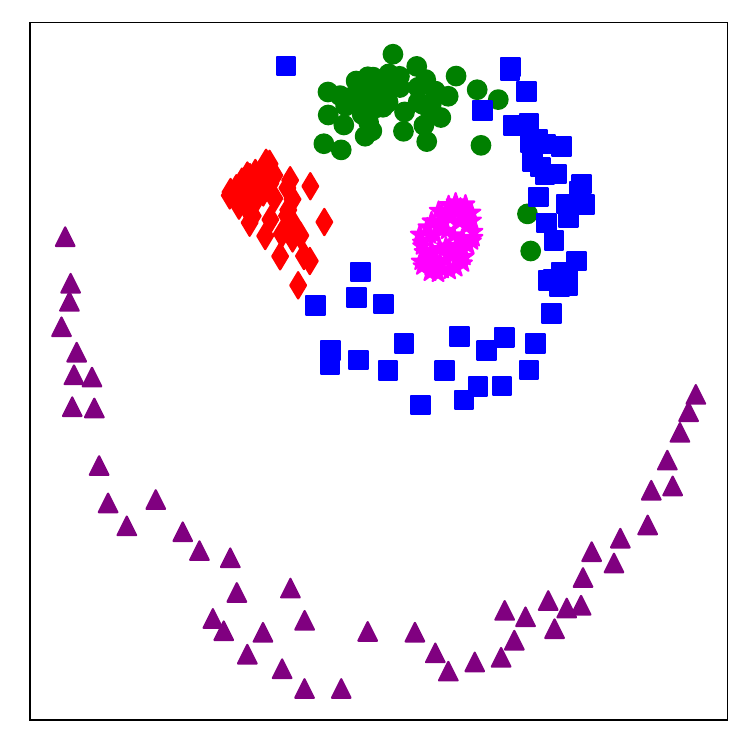}}
    \subfloat[PR18]{\includegraphics[width=0.14\textwidth]{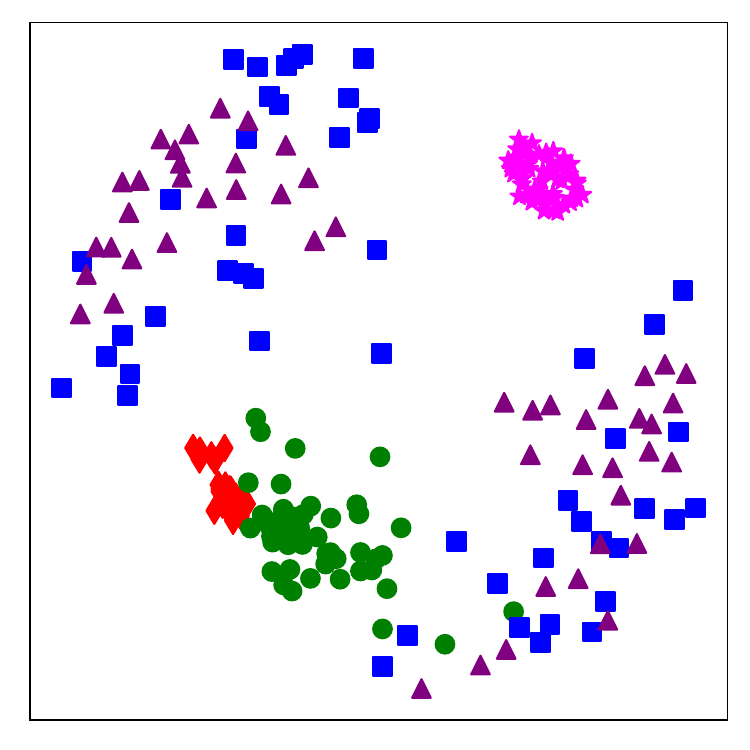}}
    \subfloat[CNN6]{\includegraphics[width=0.14\textwidth]{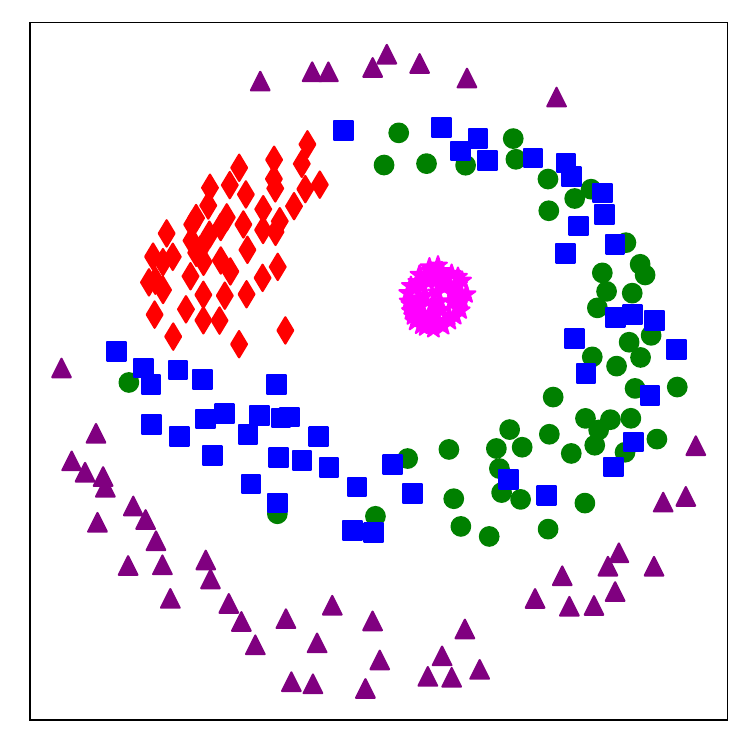}}
    \subfloat[ENet]{\includegraphics[width=0.14\textwidth]{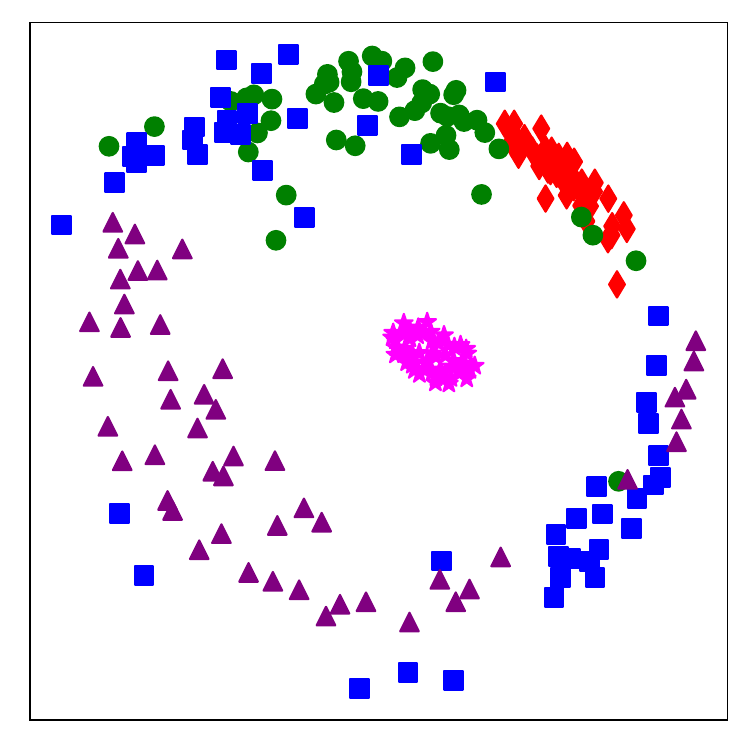}}
  \end{minipage}

    \caption{Multidimensional scaling (MDS) of cosine similarity between real latent features and random backdoor probes in 7 backdoored models poisoned with 2 different attack patterns. These models are all trained on the CIFAR10 dataset, their backdoor target is 4, and the intervals in (a-g) are their latent features' value range of random inputs.}
    \label{fig:mds}
    \vspace*{-5mm}
\end{figure*}

\begin{table*}[t]
\centering
\footnotesize
\caption{The TPR and FPR of CTell across different attacks on the full detection benchmark.}
\label{tab:attack}
\begin{tabular}{c|c|cccccccccc|c}
\toprule
Dataset& Model & Badnet & Blended & Blind & Bpp & LF & Lira & IA & ISSBA & TrojanNN & Wanet & FPR \\\hline
\multirow{6}{*}{CIFAR10} & R18  &10/10&\underline{9/10}&10/10&10/10&\underline{9/10}&10/10&10/10&\underline{9/10}&10/10&10/10&0/21\\
&PR18 &\underline{8/10} &10/10&10/10&10/10&10/10&10/10&\underline{9/10}&10/10&10/10&10/10&\underline{2/21}\\
&ENb3 &10/10 &10/10&10/10&10/10&10/10&10/10&10/10&10/10&\underline{8/10}&10/10&0/21\\
&V16 &10/10 &10/10&10/10&10/10&\underline{7/10}&\underline{8/10}&10/10&10/10&10/10&10/10&\underline{1/21}\\
&GNet &10/10 &10/10&10/10&10/10&10/10&10/10&10/10&10/10&10/10&10/10&0/21\\
&SNet &10/10 &10/10&10/10&10/10&10/10&10/10&10/10&10/10&10/10&10/10&0/21\\
&CNN6  &10/10 &10/10&10/10&\underline{6/10}&\underline{9/10}&10/10&10/10&10/10&10/10&10/10&\underline{1/21}\\\toprule
\multirow{6}{*}{GTSRB} & R18 &43/43 &43/43&43/43&43/43&43/43&43/43&43/43&43/43&43/43&43/43&0/25\\
&PR18 &43/43 &43/43&43/43&43/43&43/43&43/43&43/43&43/43&43/43&43/43&0/25\\
&ENb3 &43/43 &43/43&43/43&\underline{42/43}&43/43&43/43&43/43&43/43&43/43/&43/43&0/25\\
&V16 &\underline{40/43} &\underline{41/43}&43/43&43/43&43/43&\underline{41/43}&43/43&43/43&43/43&43/43&\underline{1/25}\\
&GNet &43/43 &43/43&43/43&43/43&43/43&43/43&43/43&43/43&43/43&43/43&0/25\\
&SNet &43/43 &43/43&43/43&\underline{41/43}&43/43&43/43&41/43&43/43&43/43&43/43&\underline{1/25}\\
&CNN6 &\underline{41/43} &\underline{40/43}&43/43&\underline{40/43}&43/43&43/43&43/43&43/43&\underline{42/43}&\underline{42/43}&\underline{1/25}\\\toprule
Dataset& Model & Badnet & Blended & Bpp & LF & IA & TrojanNN & Wanet & \multicolumn{1}{|c|}{FPR} & \multicolumn{1}{|c|}{Dataset}& Model & Badnet (TPR) \\\hline
\multirow{4}{*}{Tiny} & MV3 &40/40 &40/40&40/40&40/40&\underline{39/40}&40/40&40/40&\multicolumn{1}{|c|}{1/21}&\multicolumn{1}{|c|}{\multirow{4}{*}{MNIST}}&\multicolumn{1}{c|}{\multirow{2}{*}{LT5}}&\multirow{2}{*}{10/10}\\
&PR18 &40/40 &40/40&40/40&40/40&\underline{39/40}&40/40&40/40&\multicolumn{1}{|c|}{1/21}&\multicolumn{1}{|c|}{}&\multicolumn{1}{c|}{}&\\
&V19  &40/40&40/40&40/40&40/40&40/40&40/40&40/40&\multicolumn{1}{|c|}{0/21}&\multicolumn{1}{|c|}{}&\multicolumn{1}{c|}{\multirow{2}{*}{CNN2}}&\multirow{2}{*}{10/10}\\
&VIT &40/40&\underline{37/40}&40/40&40/40&40/40&\underline{38/40}&40/40&\multicolumn{1}{|c|}{0/21}&\multicolumn{1}{|c|}{}&\multicolumn{1}{c|}{}&\\\bottomrule
\end{tabular}
\vspace{-2mm}
\end{table*}

\subsection{Indicator Validity Analysis}
\label{apx:iva}
Besides two indicators proposed in Section \ref{sec:detectionatc}, here, we further introduce another two indicators and compare their validity:
\begin{itemize}
    \item \textbf{Class prediction proportion}:
    \begin{equation}
    \mathbf{r}^{\text{ratio}}=[r_i]_\mathcal{\mathcal{Y}}=[\frac{1}{N}\sum_{n=1}^N\mathbb{I}(\hat{y}_n=i)],
    \end{equation}
    It can intuitively reflect the model's bias towards classes. %Since random backdoor probes are isotropic or uniform, they are more likely to activate the backdoor class;
    \item \textbf{Class maximum confidence}:
    \begin{equation}
    \mathbf{r}^{\text{max}}=[z_i^{\max}]_\mathcal{\mathcal{Y}}=[\max_{n=1}^Nz_{n,i}]
    \end{equation}
    It evaluates the largest predicted logits of backdoor probes on each class. Since backdoor implantation may increase the backdoor target class's weights or bias, the target may have larger logits than other classes. %Hence, backdoor probes may achieve the largest predicted logits on the  target class.
\end{itemize}

We determine $\tau$ for four indicators using the configuration set and demonstrate their detection TPR and FPR on the full backdoor detection benchmark. We can see that due to differences in network architectures, these four indicators all have the capacity of identifying backdoor attacks to some extent, but their performance varies across different architectures and datasets. Among them, $\mathbf{r}^{\text{mean}}$ and $\mathbf{r}^{\text{l2}}$ show a better performance than others. In total, besides PreactResNet18, $\mathbf{r}^{\text{mean}}$ achieves a near-perfect and stable performance for most network architectures. Hence, we set $\mathbf{r}^{\text{mean}}$ as the detection indicator for most mdoels and only set $\mathbf{r}^{\text{l2}}$ for PreactResNet18. Note that $\mathbf{r}^{\text{ratio}}$ and $\mathbf{r}^{\text{max}}$ also have specific advantages in certain model settings. For example, $\mathbf{r}^{\text{ratio}}$ achieves an TPR of 99\% and FPR of 0\% for ENb3 on CIFAR10, better than $\mathbf{r}^{\text{mean}}$. Hence, given a small configuration set, the defender can determine which indicator should be used according to their detection accuracy.

\begin{table}[t!]
\centering
\footnotesize
\caption{The TPR and FPR (\%) of CTell across different model architectures and datasets with different indicators. The bold value is the best, while the underlined value is the second best.}
\label{tab:indicator}
\scalebox{0.96}{
\begin{tabular}{c|c|cccc}
\hline
Dataset& Model & $\mathbf{r}^{\text{ratio}}$ & $\mathbf{r}^{\text{max}}$ & $\mathbf{r}^{\text{mean}}$ & $\mathbf{r}^{\text{l2}}$ \\\hline
\multirow{7}{*}{CIFAR10} & R18  &\textbf{97/0}&89/0&\textbf{97/0}&88/0\\
&PR18 &46/14.3&32/0&96/66.7&\textbf{97/9.5}\\
&ENb3 &\textbf{99/0}&94/4.8&\underline{98/0}&\textbf{99/0}\\
&V16 &\textbf{95/4.8}&89/9.5&\textbf{95/4.8}&\textbf{95/4.8}\\
&GNet &\underline{98/9.5}&\textbf{100/0}&\textbf{100/0}&\textbf{100/0}\\
&SNet &\textbf{100/0}&75/0&\textbf{100/0}&\textbf{100/0}\\
&CNN6  &90/4.8&77/9.5&\underline{95/4.8}&\textbf{97/9.5}\\\hline
\multirow{7}{*}{GTSRB} & R18 &\textbf{100/0}&\textbf{100/0}&\textbf{100/0}&\textbf{100/0}\\
&PR18 &\underline{98.6/8}&82.1/8&\textbf{100/0}&\textbf{100/0}\\
&ENb3 &\textbf{99.8/0}&\textbf{99.8/0}&\textbf{99.8/0}&\textbf{99.8/0}\\
&V16 &93.5/8&72.6/0&\textbf{98.4/4}&\underline{98.1/4}\\
&GNet &\textbf{100/0}&\textbf{100/0}&\textbf{100/0}&\textbf{100/0}\\
&SNet &\textbf{99.1/4}&85.3/0&\textbf{99.1/4}&\textbf{99.1/4}\\
&CNN6 &97.9/8&89.8/8&\underline{97.9/4}&\textbf{97.9/0}\\\hline
\multirow{4}{*}{Tiny} & MV3 &96.1/9.5&67.9/0&\textbf{99.6/4.8}&\underline{96.4/4.8}\\
&PR18 &91.1/9.5&65.4/0&\underline{98.9/9.5}&\textbf{99.6/4.8}\\
&V19 &\textbf{100/0}&97.9/9.5&\textbf{100/0}&\textbf{100/0}\\
&VIT &\underline{96.8/4.8}&47.1/9.5&\textbf{98.2/0}&93.9/0\\\hline

\multirow{2}{*}{MNIST} & LT5 &\textbf{100/0}&100/90&\textbf{100/0}&\textbf{100/0}\\
&CNN2 &100/20&80/0&\textbf{100/0}&\textbf{100/0}\\\hline
Overall & & 96.49/4.9 &83.71/13.0&\textbf{98.99}/5.2 & \underline{98.47}/\textbf{2.1}\\\hline
\end{tabular}
}

\vspace{-3mm}
\end{table}

\subsection{Detection Performance under different attacks}
\label{apx:configuration}
Table \ref{tab:attack} illustrates the details of CTell's TPR and FPR against different backdoor attacks across different classes. Class imbalance is a well-known issue in machine learning tasks. This issue can result in imbalanced decision spaces between different classes. The class with more feature distributions often has a greater decision space, which will also lead to our backdoor probes being trapped in. Backdoor attacks introduce additional trigger features to the backdoor class, causing this imbalance to tilt towards the class. And because the trigger itself typically has a big difference from the benign features of the backdoor class (they are typically orthogonal \cite{zhang2024exploring, wang2022rethinking}), this imbalance is more prominent. Our approach takes advantage of this essence. In Table \ref{tab:attack}, we can see that across different attacks, model architectures, datasets, and their classes, CTell can identify the backdoor attacks in most cases.

% \end{appendices}
